# Supplementary material for: Flexibility of Integrated Power and Gas Systems: Gas Flow Modeling and Solution Choices Matter
Source: arXiv:2311.05744 source file (2024-11-18)
Supplement: Supplementary file 1 [file 07_Appendix_PDE.tex]

\section{Original gas flow equations}
\label{section:appendix_PDE}
\setcounter{equation}{0}

The one-dimensional dynamic flow of natural gas along the pipeline axis is governed by a set of nonlinear and nonconvex PDEs, named Euler's equations \eqref{eq:A1}-\eqref{eq:A3} \cite{lurie2009modeling}: 
\begingroup
\allowdisplaybreaks
\begin{align}
    &\frac{\partial \rho}{\partial t} + \frac{\partial (\rho u)}{\partial x}= 0 \label{eq:A1} \\
    & \frac{\partial (\rho u)}{\partial t} + \frac{\partial \pi}{\partial x} + \frac{\partial (\rho u^2)}{\partial x} +\rho g \sin\alpha + \lambda \frac{\rho u |u|} {2D} = 0 \label{eq:A2} \\
    & \frac{\partial}{\partial t} \left[\rho \left(e+\frac{1}{2}u^2 \right) \right]+\frac{\partial}{\partial x} \left[(\rho u) \left(h+\frac{1}{2}u^2 \right)\right] \notag\\
    &-\rho \Omega +\rho g u \sin\alpha  = 0, \label{eq:A3} 
\end{align}
where $t$ and $x$ represent the time and space dimensions. The symbols $\rho$, $u$, and $\pi$ describe the density, velocity, and pressure of the natural gas, respectively. Pipeline-specific constants $D$, $\alpha$, and $\lambda$ denote the diameter, inclination angle, and friction factor\footnote{The friction factor is a function of the pipeline characteristics (i.e., diameter, roughness, and Reynolds number). For natural gas transmission pipelines, it can be calculated with the Colebrook-White equation for turbulent flow since the Reynolds number of the gas is high enough \cite{Menon}.} of the pipeline's inner walls. Constant $g$ denotes the acceleration of gravity. The symbols $e$ and $h$ represent the specific internal energy and enthalpy of the gas, respectively, whereas $\Omega$ is the heat transfer rate per unit of time and mass. The continuity equation \eqref{eq:A1} describes the principle of conservation of mass in a differential form, stating that the net mass rate flowing outside a differential gas volume is equal to the rate of decrease in the mass present within the differential volume \cite{Liu2011}. The conservation of momentum equation \eqref{eq:A2} represents the differential form of Newton’s second law, stating that, at each time instant, the sum of all forces exerted on a fluid volume is equal to the rate of increase in momentum. The forces appearing in equation \eqref{eq:A2} are: the natural gas \textit{inertia term} $\frac{\partial (\rho u)}{\partial t}$, the \textit{pressure gradient} along the axis $\frac{\partial \pi}{\partial x}$, the advection term $\frac{\partial (\rho u^2)}{\partial x}$ (also referred to as the kinetic energy term), the force of gravity $\rho g \sin\alpha $, and the \textit{friction force} $\lambda \frac{\rho u |u|} {2D} $.  Finally, \eqref{eq:A3} enforces energy conservation in differential form. In addition to those three PDEs, the equation of state relates the gas state variables (i.e., density, pressure, and temperature):
\begin{equation}
    \pi = \frac{Z(\pi,T) R T}{M_g}\rho, \label{eq:A4}
\end{equation}
where $Z$ is the natural gas compressibility factor, which is a function of pressure and temperature, $R$ is the universal gas constant, $T$ is the absolute temperature, and $M_g$ is the molecular weight of natural gas.

For high-pressure natural gas transmission pipelines, the following three assumptions are generally adopted to simplify Equations~\eqref{eq:A1}--\eqref{eq:A4}:
\begin{enumerate}
    \item In \eqref{eq:A2}, the advection term $\frac{\partial (\rho u^2)}{\partial x}$ and the impact of non-horizontal pipelines $\rho g \sin\alpha $ are negligible compared to the pressure gradient $\frac{\partial \pi}{\partial x}$ \cite{correa2014pw, Liu2011}, and therefore dropped.
    \item Flow is assumed to be isothermal, meaning the temperature is constant and the pipeline is in thermal equilibrium with the environment ($\Omega=0$) \cite{Liu2011, Wei2020book,  correa2014pw}. Consequently, \eqref{eq:A3} can be neglected.
    \item In~\eqref{eq:A4}, the compressibility factor is assumed to be constant in both temperature (following the isothermal flow assumption) and pressure.
    This implies a direct proportionality between gas pressure and density, which simplifies~\eqref{eq:A4} to $\pi = c^2 \rho$, %\label{eq:A5}
    where $c$ is the speed of sound in gas and is defined as $c^2 = \frac{Z R T}{M_g}$.
\end{enumerate}
By using the cross-sectional pipeline area $A$, introducing the mass flow $m=\rho u A$, and applying the simplifying assumptions above, \eqref{eq:A1}-\eqref{eq:A4} can be rewritten as:
\begingroup
\allowdisplaybreaks
\begin{align}
    & \hspace{11pt} \frac{\partial \pi}{\partial t} + \frac{c^2}{A}\frac{\partial m}{\partial x} = 0 \label{eq:A5} \\
    & \underbrace{\frac{\partial m}{\partial t}}_\text{Inertia term} + \underbrace{A \frac{\partial \pi}{\partial x}}_\text{Pressure gradient} + \underbrace{\frac{\lambda c^2}{2DA} \frac{m |m|} {\pi}}_\text{Friction force} = 0. \label{eq:A6}
\end{align}
