# Supplementary material for: Flexibility of Integrated Power and Gas Systems: Gas Flow Modeling and Solution Choices Matter
Source: arXiv:2311.05744 source file (2024-11-18)
Supplement: Supplementary file 2 [file 09_Appendix_models.tex]

\section{Solution choices continued}
\label{section:appendix_model}
\setcounter{equation}{0}

This section contains a detailed explanation of individual parameters and additional information on some of the solution choices presented in Section~\ref{section:04_NGsol} of the main paper.

\subsection{Mixed-integer linear relaxation}
\label{sec:MILP_app}
It has been proposed in \cite{ORDOUDIS2019} to choose the set of linearization points based on a uniform grid over the feasible region of the flow and pressure variables. This approach neglects the curvature of the function and may yield a low approximation accuracy at some points. Instead, we follow the same approach to deriving the polyhedral envelopes introduced in Sections~IV.F and \ref{sec:PELP_app}. To account for the modeling of the flow direction using the binary variable $z$ and nonnegative auxiliary variables $\gamma^{+/-}$ and $m^{+/-}$, we divide the polyhedral envelopes resulting from the linearization points in~\eqref{eq:polyhedral_envelops} into positive and negative flow direction. For envelopes $u = \{1,2,3\}$, we replace $\gamma$ and $m$ by $m^+$ and $\gamma^+$. Similarly, for envelopes $u = \{4,5,6\}$, we replace $\gamma$ and $m$ by $m^-$ and $\gamma^-$. Additionally, we switch the signs of $\underline{M}$ to account for the nonnegativity of the flow.

The feasible region of $\mathrm{MILP}$ is substantially reduced compared to the $\mathrm{PELP}$ by including the flow directions as binary variables (see Fig.~4). To further strengthen the relaxation, we derive one additional halfspace per flow direction based on the intersection of the planes defined by $u=1$ and $u=4$ with nonnegativity $\gamma^+ \geq 0$ and $\gamma^- \geq 0$, respectively. Analogously to the derivation of the linearization points $\widetilde{m}^3$ and $\widetilde{m}^6$, we derive those points by fixing $\pi = \widehat{\Pi}_{ij}^{+}$ and $\pi = \widehat{\Pi}_{ij}^{-}$, respectively, and projecting the intersection point on the manifold. The flow of the resulting linearization points $u=7$ for $m^+$ and $u=8$ for $m^-$ are then given by
\begin{align}
    \widetilde{m}^{7} = \frac{(\sqrt{8}-3) \cdot \overline{M}}{2-\sqrt{8}}, \\
    \widetilde{m}^{8} = \frac{(\sqrt{8}-3) \cdot \underline{M}}{2-\sqrt{8}}.
\end{align}

\subsection{Polyhedral envelopes}
\label{sec:PELP_app}
We generally follow the approach presented in \cite{Mhanna2022} to derive the sets of linearization points $u \in \mathcal{U}$ and $o \in \mathcal{O}$, where $|\mathcal{U}| = |\mathcal{O}| = 3$. The sets $\mathcal{U}$ and $\mathcal{O}$ are used to derive under- and over-estimators, respectively. While \cite{Mhanna2022} derives individual polyhedral envelopes for both sides of the Weymouth equation~\eqref{eq:weymouth}, we directly derive it for the three-dimensional function in~\eqref{eq:gamma_def}, by fixing the average pipeline pressure $\pi$ to a predefined value. We observed that the maximum value of $\gamma$ is attained at the maximum pipeline pressure difference (see Section~V.A). Therefore, we use $\widetilde{\pi}^u =  \widehat{\Pi}_{ij}^{+}$ for $u = \{1,2,3\}$ and $\widetilde{\pi}^o =  \widehat{\Pi}_{ij}^{-}$ for $o = \{4,5,6\}$. The corresponding points of the mass flow $\widetilde{m}^u$, for $u = 1,2,3$, and $\widetilde{m}^o$, for $o = 4,5,6$, are given by
\begin{align}\label{eq:polyhedral_envelops}
    &\widetilde{m}^{1} = (1-\sqrt{2})\cdot\underline{M}, &\, &\widetilde{m}^{4} = (1-\sqrt{2})\cdot\overline{M}  \\
    &\widetilde{m}^{2} = \overline{M}, &\, &\widetilde{m}^{5} = \underline{M} \\
    &\widetilde{m}^{3} = \frac{-\underline{M}^2 (\sqrt{8}-3) - \overline{M}^2}{\underline{M} (2-\sqrt{8}) - 2 \overline{M}}, &\, &\widetilde{m}^{6} = \frac{\underline{M}^2 (3-\sqrt{8}) + \overline{M}^2}{\overline{M} (\sqrt{8}-2) + 2 \underline{M}}.
\end{align}
We refer the interested reader to \cite{Mhanna2022} for a more detailed elaboration on deriving the individual linearization points.
