# Supplementary material for: Flexibility of Integrated Power and Gas Systems: Gas Flow Modeling and Solution Choices Matter
Source: arXiv:2311.05744 source file (2024-11-18)
Supplement: Supplementary file 3 [file 12_Appendix_LargeCase.tex]

\section{Case Study B: Large-scale integrated power and gas system}
\label{section:appendix_case_study}
\setcounter{equation}{0}

% To analyze the impact of the considered solution choices on a realistic large-scale integrated power and gas system, we consider Case Study B, which is a modified version of the GasLib 40-node gas network \cite{GasLib} connected to a modification of the 24-bus IEEE RTS power system in \cite{ordoudis2016updated}. A schematic diagram of the integrated system is shown in Figure~\ref{fig:large_case}.
% % %
% \input{tikz/large_case_15km}
% %

Case Study B is a modified version of the GasLib 40-node gas network \cite{GasLib} connected to a modification of the 24-bus IEEE RTS power system in \cite{ordoudis2016updated}. In the following, we describe the modifications we performed on the gas network.
To avoid circular gas flows arising from the neglection of operational states of the compressors, innode 3 and pipelines 33 and 39 have been removed from the gas network.
We set a pressure range of \qty{31}-\qty{81}{\bar} for all nodes. The pressure at source nodes before compressors is fixed such that the maximum nodal pressure at the compressor outlet is met at full compression. Given a maximum compression ratio of \qty{1.5}, this is around \qty{54}{\bar}.
We use the same profiles shown in Fig.~2 of the main paper for all electrical loads, gas loads, and wind farms, varying their peak load and installed capacity, respectively.
The data can be found in the GitHub repository \cite{Online_Companion}. We consider the $\mathrm{DY}$ model only and apply a time and space discretization of \qty{15}{\minute} and \qty{15}{\kilo\meter}, respectively.
Except for solution choices $\mathrm{NLP}$, $\mathrm{SLP}$, and $\mathrm{PELP}$, no other method was able to solve the OPGF problem within \qty{24}{\hour}.

% The different colors of the pipelines in Figure~\ref{fig:large_case} illustrate each pipeline's root mean squared (RMS) relaxation gap. This is done by calculating $\Phi^{\mathrm{RMS}}$ according to Equation~\eqref{eq:gap_rms} for each pipeline $(i,j)$ using the stacked relative relaxation gaps $\mathbf{\Phi}_{ij}$ and without normalizing by the square-root of the total number of pipelines.  Generally, it can be observed that the relaxation gap is, on average, higher around junctions. Assuming, e.g., gas flows from a junction into two pipelines with the same pressure gradient. Then, the relaxation gap can be utilized to have a proportionally lower flow on one of the connected branches. For solution choices $\mathrm{MILP}$ and $\mathrm{PELP}$, an over proportionally high flow compared to the pressure gradient could also be feasible. However, since the pressure ranges are usually nonbinding, this rarely happens, as a larger pressure gradient could be chosen. 
